# Supplementary material for: TensorQuant - A Simulation Toolbox for Deep Neural Network Quantization
Source: arXiv:1710.05758 source file (2017-10-13)
Supplement: Supplementary file 1 [file Appendix.tex]

\section*{Appendix}

\begin{lstlisting}[caption={Layer factory for convolution type layers.}, label{lst:layer_factory}]
def conv2d_factory(intr_q_map=None, extr_q_map=None):
def func(*args,**kwargs):
layer_ID=tf.get_variable_scope().name+
"/"+kwargs["scope"]
if intr_q_map is None:
net=slim.conv2d(*args,**kwargs)
elif ("conv2d" in intr_q_map.keys() or
any(layer in layer_ID for layer in intr_q_map.keys()) 
):
layer=next(layer for layer in intr_q_map.keys() if(
layer in layer_ID or layer=="conv2d") )
kwargs['quantizer']=intr_q_map[layer]
net=QConv.conv2d(*args,**kwargs)
else:
net=slim.conv2d(*args,**kwargs)

if extr_q_map is None:
return net
elif ("conv2d" in extr_q_map.keys() or
any(layer in layer_ID for layer in extr_q_map.keys()) 
):
layer=next(layer for layer in extr_q_map.keys() if(
layer in layer_ID or layer=="conv2d") )
return extr_q_map[layer].quantize(net)
else:
return net   
return func
\end{lstlisting}
